# Supplementary material for: Loss Balancing for Fair Supervised Learning
Source: arXiv:2311.03714 source file (2023-11-07)
Supplement: Supplementary file 1 [file appendix.tex]

\section{Appendix}
\subsection{Proofs}

In order to prove Theorem \ref{theo:main},  we first introduce two lemmas. 

\begin{lemma}\label{lem1}
Under assumption \ref{assump:2}, there exists $\overline{\pmb{w}} \in \mathbb{R}^{d_{w}}$ such that $L_0(\overline{\pmb{w}}) = L_1(\overline{\pmb{w}}) = L(\overline{\pmb{w}})$ and $\lambda^{(1)}_{start} \leq L(\overline{\pmb{w}}) \leq \lambda^{(1)}_{end}$.
\end{lemma}

\textbf{Proof.} Let $h_0(\beta) = L_0((1-\beta)\pmb{w}_{G_0} + \beta \pmb{w}_{G_1})$ and  $h_1(\beta) = L_1((1-\beta)\pmb{w}_{G_0} + \beta \pmb{w}_{G_1})$, and $ h(\beta) = h_0(\beta) - h_1(\beta), \beta \in [0,1]$. Note that $\nabla_{\pmb{w}} L_a( \pmb{w}_{G_a}  ) = 0$ because $\pmb{w}_{G_a}$ is the minimizer of $L_a( \pmb{w}  )$. Moreover, $ \nabla^2_{\pmb{w}} L_a( \pmb{w}   )$ is positive semi-definit because $L_a(.)$ is a strictly convex function.  

First, we show that $L_0((1-\beta)\pmb{w}_{G_0} + \beta \pmb{w}_{G_1})$ is an increasing function in $\beta$, and $L_1((1-\beta)\pmb{w}_{G_0} + \beta \pmb{w}_{G_1})$ is a decreasing function in $\beta$. Note that $h'_0(0) = (\pmb{w}_{G_1}-\pmb{w}_{G_0})^T  \nabla_{\pmb{w}} L_0( \pmb{w}_{G_0}  )  = 0$,  and $h''_0(0) = (\pmb{w}_{G_1}-\pmb{w}_{G_0})^T  \nabla^2_{\pmb{w}} L_0( \pmb{w}_{G_0}  ) (\pmb{w}_{G_1}-\pmb{w}_{G_0}) \geq 0 $. This implies that $h'_0(\beta) \geq 0, \forall \beta\in [0,1]$. Similarly, we can show that $h'_1(\beta)\leq 0, \forall \beta \in [0,1]$.  

Note that under Assumption \eqref{assump:2}, $h(0) <0$ and $h(1)>0$. Therefore, by the intermediate value theorem, the exists $\overline{\beta}\in (0,1)$ such that $h(\overline{\beta}) = 0$. Define $\overline{\pmb{w}} = (1-\overline{\beta})\pmb{w}_{G_0} + \overline{\beta}\pmb{w}_{G_1} $. We  have,

\begin{eqnarray*}
h(\overline{\beta}) &=& 0 \implies L_0(\overline{\pmb{w}}) = L_1(\overline{\pmb{w}}) = L(\overline{\pmb{w}})\\
\pmb{w}_{G_0} &\mbox{is}& \mbox{minimizer of } L_0 \implies\\ L(\overline{\pmb{w}})&=& L_0(\overline{\pmb{w}}) \geq \lambda^{(1)}_{start}\\
h'_0 (\beta) &\geq& 0, \forall \beta\in[0,1] \implies h_0(1) \geq h_0(\overline{\beta}) \implies\\ \lambda_{end}^{(1)} &\geq& L_0(\overline{\pmb{w}}) = L(\overline{\pmb{w}})
\end{eqnarray*}
 
 \begin{lemma}\label{lem2}
 $L_0(\pmb{w}_i^*) = \lambda_{mid}^{(i)}$, where $\pmb{w}_i^*$ is the solution to \eqref{eq:OptAlg}.
 \end{lemma}
 
 \textbf{Proof.} We proceed by contradiction. Assume that $L_0(\pmb{w}_i^*)<\lambda_{mid}^{(i)}$ (i.e., $\pmb{w}_i^*$ is an interior point of the feasible set of \eqref{eq:OptAlg}). Notice that $\pmb{w}_{G_1}$ cannot be  in the feasible set of \eqref{eq:OptAlg} because $L_0(\pmb{w}_{G_1}) = \lambda_{end}^{(0)} > \lambda_{mid}^{(i)}$. As a result, $\nabla_{\pmb{w}} L_1(\pmb{w}_i^*) \neq0$. This is a contradiction because $\pmb{w}_i^*$ is an interior point of the feasible set of a convex optimization and cannot be optimal if $\nabla_{\pmb{w}} L_1(\pmb{w}_i^*)$ is not equal to zero. 

\textbf{Proof [Theorem \ref{theo:main}]}

Let $I_i = [\lambda_{start}^{(i)},\lambda^{(i)}_{end}]$ be a sequence of intervals. It is easy to see that $I_1\supseteq I_2\supseteq \cdots $ and $ \lambda^{(i)}_{end} -\lambda_{start}^{(i)} \to 0$ as $i\to \infty$. Therefore, by the Nested Interval Theorem, $\cap_{i=1}^{\infty} I_i$ consists of exactly one real number $\lambda^*$, and both $\lambda_{start}^{(i)}$ and $\lambda_{end}^{(i)}$  converge to $\lambda^*$. Because $\lambda_{mid}^{(i)} = \frac{\lambda_{start}^{(i)} + \lambda_{start}^{(i)}}{2}$, $\lambda_{mid}^{(i)}$ also converges to $\lambda^*$. 

Now, we show that $L(\w^*)\in I_i$ for all $i$. Note that $L(\w^*)= L_0(\w^*) \geq \lambda_{start}^{(1)}$ because $\pmb{w}_{G_0}$ is the minimizer of $L_0$. Moreover, $\lambda_{end}^{(1)}\geq L(\w^*)$ otherwise $L(\overline{\pmb{w}})< L(\w^*)$ ($\overline{\pmb{w}}$ is defined in Lemma \ref{lem1}) and $\w^*$ is not optimal solution under 0-EL. Therefore, $L(\w^*)\in I_1$. 

Now we proceed by induction. Suppose $L(\w^*)\in I_i$. We show that $L(\w^*) \in I_{i+1}$ as well. We consider two cases. 
\begin{itemize}
\item $L(\w^*)\leq \lambda_{mid}^{(i)}$. In this case $\w^*$ is a feasible point for \eqref{eq:OptAlg}, and $L_i(\w_i^*)=\lambda^{(i)}\leq L(\w^*)\leq \lambda_{mid}^{(i)}$. Therefore, $L(\w^*)\in I_{i+1}$.

\item $L(\w^*)> \lambda_{mid}^{(i)}$. In this case, we proceed by contradiction to show that $\lambda^{(i)} \geq \lambda_{mid}^{(i)}$. Assume that $\lambda^{(i)}<\lambda_{mid}^{(i)}$. Define $g(\beta) = g_0(\beta) - g_1(\beta)$, where $g_i(\beta) = L_i((1-\beta)\pmb{w}_{G_0} + \beta \pmb{w}_i^*)$. Note that $\lambda^{(i)} = g_1(1)$ By Lemma \ref{lem2}, $g_0(1) = \lambda_{mid}^{(i)}$. Therefore, $g(1) = \lambda_{mid}^{(i)} - \lambda^{(i)}>0$. Moreover, under Assumption \ref{assump:2}, $g(0)<0$. Therefore, by the intermediate value theorem, there exists $\overline{\beta}\in (0,1)$ such that $g(\overline{\beta}) = 0$. Similar to the proof of Lemma \ref{lem1}, we can show that $g_0(\beta)$ in an increasing function for all $\beta \in [0,1]$. As a result $g_0(\overline{\beta}) <g_0 (1) = \lambda_{mid}^{(i)}$. Define $\overline{\pmb{w}} = (1-\overline{\beta})\pmb{w}_{G_0} + \overline{\beta} \pmb{w}_i^*$. We have, 
\begin{eqnarray}
g_0(\overline{\beta}) = L_0(\overline{\pmb{w}}) = L_1(\overline{\pmb{w}}) = L(\overline{\pmb{w}}) < \lambda_{mid}^{(i)}\\
L(\w^*)> \lambda_{mid}^{(i)}
\end{eqnarray}
The last two equations imply that $\w^*$ is not an optimal fair solution under $0$-EL fairness constraint. This is a contradiction. Therefore, if $L(\w^*)> \lambda_{mid}^{(i)}$, then   $\lambda^{(i)} \geq \lambda_{mid}^{(i)}$. As a result, $L(\w^*) \in I_{i+1}$
\end{itemize} 

By the two above cases and the nested interval theorem, we conclude that, 

$$ L(\w^*) \in \cap_{i=1}^{\infty} I_i, ~ \lim_{i\to \infty} \lambda_{mid}^{(i)} = L(\w^*)$$

For the second part of the theorem, consider the following,

$$\pmb{w}_{\infty}^*  = \arg\min_{\pmb{w}} L_1(\pmb{w}) s.t., L_0(\pmb{w}) \leq \lambda_{mid}^{\infty} = L(\w^*)$$

$$\lim_{i\to \infty} \pmb{w}_i^* = \pmb{w}_{\infty}^*$$

By lemma \ref{lem2}, $L_0(\w_{\infty}^*) =  \lambda_{mid}^{\infty} = L(\w^*)$. Therefore, $L_0(\w_{\infty}^*)=L_1(\w_{\infty}^*) $, and $\w_{\infty}^*$ is the solution to optimization problem \eqref{eq:mainOP}.
%In order to show that $\w^*_{\infty}$ is equal to $\w^*$, we proceed by contradiction. Suppose $\pmb{w}^*_{\infty} \neq \w^*$. As a result, $L_1(\pmb{w}^*_{\infty})< L(\w^*)$.
% Define $\eta(\beta) = \eta_0(\beta) - \eta_1(\beta)$, where $\eta_i(\beta) = L_i((1-\beta)\pmb{w}_{G_0} + \beta \pmb{w}_{\infty}^*)$. Note that $L_1(\pmb{w}^*_{\infty}) = \eta_1(1)$. By Lemma \ref{lem2}, the condition in \eqref{eq:OptAlg} is binding and $\eta_0(1) = L(\w^*)$. Therefore, $\eta(1) = L(\w^*) - L_1(\pmb{w}^*_{\infty})>0$. Moreover, under Assumption \ref{assump:2}, $\eta(0)<0$. Therefore, by the intermediate value theorem, there exists $\overline{\beta}\in (0,1)$ such that $\eta(\overline{\beta}) = 0$. Similar to the proof of Lemma \ref{lem1}, we can show that $\eta_0(\beta)$ is an increasing function for all $\beta \in [0,1]$. As a result $\eta_0(\overline{\beta}) <\eta_0 (1) = L(\w^*)$. Define $\overline{\pmb{w}} = (1-\overline{\beta})\pmb{w}_{G_0} + \overline{\beta} \pmb{w}_\infty^*$. We have, 
% \begin{eqnarray}
%\eta_0(\overline{\beta}) = L_0(\overline{\pmb{w}}) = L_1(\overline{\pmb{w}}) = L(\overline{\pmb{w}}) < L(\w^*)
%\end{eqnarray}
%The last equation implies that $\w^*$ is not an optimal fair solution under $0$-EL fairness constraint. This a contradiction. As a result, $\pmb{w}_{\infty}^* = \pmb{\hat{w}}$. 

\textbf{Proof [Theorem \ref{theo:gammaEL} ]}

Let $\pmb{w}^*$ be the optimal weight vector under $\gamma$-EL. 

\textbf{Step 1.} we show that one of the following holds, 
\begin{eqnarray}
L_0(\pmb{w}^*) - L_1(\pmb{w}^*) = \gamma \\
L_0(\pmb{w}^*) - L_1(\pmb{w}^*) = -\gamma 
\end{eqnarray}
Proof by contradiction. Assume $-\gamma < L_0(\pmb{w}^*) - L_1(\pmb{w}^*) <\gamma$. This implies that $\pmb{w}^*$ is an interior point of the feasible set of optimization problem \eqref{eq:mainOP}.  Since $\pmb{w}^* \neq \pmb{w}^*_{O}$, then $\nabla L(\pmb{w}^*) \neq 0$. As a result, object function of \eqref{eq:mainOP} can be improved at $\pmb{w}^*$ by moving toward $-\nabla L(\pmb{w}^*)$. This a contradiction. Therefore,  $|L_0(\pmb{w}^*) - L_1(\pmb{w}^*)| = \gamma$.

\textbf{Step 2.} Function $\pmb{w}_{\gamma} = \texttt{ELminimizer}(\pmb{w}_{G_0},\pmb{w}_{G_0},\epsilon,\gamma)$ is the solution to the following optimization problem, 
\begin{eqnarray}\label{eq:plusgamma}
 \min_{\pmb{w}} \Pr\{A=0\} L_0(\pmb{w}) + \Pr\{A=1\}L_1(\pmb{w}),\nonumber\\ s.t., L_0(\pmb{w}^*) - L_1(\pmb{w}^*) = \gamma
\end{eqnarray}
 
 To show the above claim, notice that the solution to optimization problem  \eqref{eq:plusgamma} is the same as the following, 
 
 \begin{eqnarray}\label{eq:plusgamma2}
 \min_{\pmb{w}} \Pr\{A=0\} L_0(\pmb{w}) + \Pr\{A=1\}\tilde{L}_1(\pmb{w}),\nonumber\\ s.t., L_0(\pmb{w}^*) - \tilde{L}_1(\pmb{w}^*) = 0,
\end{eqnarray}
where $\tilde{L}_1(\w) = L_1(\w) + \gamma$.
Since $L_0(\w_{G_0}) - \tilde{L}_1(\w_{G_0})<0 $ and $L_0(\w_{G_1}) - \tilde{L}_1(\w_{G_1})>0 $, by Theorem \ref{theo:main}, we know that $\w_{\gamma} = \texttt{ELminimizer}(\pmb{w}_{G_0},\pmb{w}_{G_0},\epsilon,\gamma)$ find the solution to \eqref{eq:plusgamma2}. 

Lastly, because $|L_0(\pmb{w}^*) - L_1(\pmb{w}^*)| = \gamma$, we have, 

\begin{eqnarray}
\w^* = \left\lbrace \begin{array}{ll} \w_\gamma & \mbox{if } L(\w_\gamma) \leq L(\w_{-\gamma})\\
\w_{-\gamma} & \mbox{o.w.}\end{array} \right.
\end{eqnarray}
Thus, Algorithm \ref{Alg2} finds the solution to \eqref{eq:mainOP}. 

\textbf{Proof [Theorem \ref{Theo:3}]}

\begin{enumerate}
\item Under Assumption \ref{assump:2}, $g(1)<0$. Moreover, $g(0) \geq 0$. Therefore, by the intermediate value theorem, there exists $\beta_0\in [0,1]$ such that $g(\beta_0) = 0$. 

\item Since $\w_O$ is the minimizer of $L(\w)$, $h'(0) = 0$. Moreover, since $L(\w)$ is strictly convex, $h''(0)>0$. As a result, $h'(\beta)>0$ for  $\beta>0$. 

\item Since $\w_{G_{\hat{a}}}$ is the minimizer of $L_{\hat{a}}(\w)$, and $L_{\hat{a}}(\w)$ is strictly convex,  $ L_{\hat{a}}((1-\beta) \pmb{w}_O + \beta \w_{G_{\hat{a}}}) $ is strictly decreasing function. 

Note that since $h(\beta) = \Pr\{A=\hat{a}\} L_{\hat{a}}((1-\beta) \pmb{w}_O + \beta \w_{G_{\hat{a}}}) + \Pr\{A=1-\hat{a}\} L_{1-\hat{a}}((1-\beta) \pmb{w}_O + \beta \w_{G_{\hat{a}}})$ is strictly increasing and $ L_{\hat{a}}((1-\beta) \pmb{w}_O + \beta \w_{G_{\hat{a}}}) $ is strictly decreasing, we conclude that $L_{1-\hat{a}}((1-\beta) \pmb{w}_O + \beta \w_{G_{\hat{a}}})$ is strictly increasing. As a result, $g$ should be strictly decreasing.

\end{enumerate}

\textbf{Proof [Theorem \ref{theo:sub}]}
First, we show that if $g_{\gamma}(0) \leq 0$, then $\w_O$ satisfies $\gamma$-\textsf{EL}.

$$g_{\gamma}(0)\leq 0 \implies g(\beta) - \gamma \leq 0 \implies L_{\hat{a}}(\w_O) - L_{1-\hat{a}}(\w_O) \leq \gamma$$

Moreover, $L_{\hat{a}}(\w_O) - L_{1-\hat{a}}(\w_O)\geq 0$ because $\hat{a} = \arg\max_a L_a(\w_O)$.  Therefore, $\gamma$-\textsf{EL} is satisfied. 

Secondly, assume that $g_{\gamma}(0) > 0$. Under Assumption 1, $g_{\gamma}(1) = L_{\hat{a}}(\w_{G_{\hat{a}}}) - L_{1-\hat{a}}(\w_{G_{\hat{a}}}) -\gamma <0 $. Therefore, by the intermediate value there exists $\beta_0$ such that $g_{\gamma}(\beta_0) = 0$. Moreover, $g_{\gamma}$ is a strictly decreasing function. Therefore, the binary search proposed in Algorithm 3 converges to root of $g_{\gamma}(\beta)$.  As a result, $(1-\beta_{mid}^{(\infty)})\w_O + \beta_{mid}^{(\infty)} \w_{G_{\hat{a}}}$ satisfies  satisfies $\gamma$-\textsf{EL}.  Moreover, $L_{\hat{a}}(\w_O) - L_{1-\hat{a}}(\w_O)\geq 0$ because $\hat{a} = \arg\max_a L_a({\w}_O)$. Note that since $g(\beta)$ is decreasing, $\beta^{(\infty)}_{mid}$ is the smallest possible $\beta$ under which $(1-\beta)\w_O + \beta \w_{G_{\hat{a}}}$ $\gamma$-\textsf{EL}. Since $h$ is increasing,  the smallest possible  $\beta$ gives us a better accuracy.

\textbf{Proof [Theorem \ref{theo:learnable}]} 

By the triangle inequality, the following holds, 

\begin{eqnarray}
\sup_{f_{\pmb{w}}\in \mathcal{F}} | |L_0(\pmb{w}) - L_1(\pmb{w}) | - |\hat{L}_0(\pmb{w}) - \hat{L}_1(\pmb{w})| | \leq \\ \sup_{f_{\pmb{w}}\in \mathcal{F}} |L_0(\pmb{w}) - \hat{L}_0(\pmb{w})| + \sup_{f_{\pmb{w}}\in \mathcal{F}} |L_1(\pmb{w}) - \hat{L}_1(\pmb{w})|.
\end{eqnarray}
Therefore, with probability at least $1-2\delta$ we have, 
 \begin{eqnarray}
 \label{eq:ineq}
 \sup_{f_{\pmb{w}}\in \mathcal{F}} | |L_0(\pmb{w}) - L_1(\pmb{w}) | - |\hat{L}_0(\pmb{w}) - \hat{L}_1(\pmb{w})| | \leq \nonumber \\ B(\delta,n_0,\mathcal{F}) + B(\delta,n_1,\mathcal{F})
 \end{eqnarray}
 As a result, with probability $1-2\delta$ holds,
 \begin{eqnarray}\label{eq:subset}
 \{\pmb{w}| f_{\pmb{w}} \in \mathcal{F}, |L_0(\pmb{w}) - L_1(\pmb{w}) |\leq \gamma\} \subseteq\nonumber \\  \{\pmb{w}| f_{\pmb{w}} \in \mathcal{F}, |\hat{L}_0(\pmb{w}) - \hat{L}_1(\pmb{w}) |\leq \hat{\gamma}\}
 \end{eqnarray}
 Now consider the following, 

 \begin{equation}
L(\pmb{\hat{w}}) -  L(\pmb{w}^*) = L(\pmb{\hat{w}}) - \hat{L}(\pmb{\hat{w}}) + \hat{L}(\pmb{\hat{w}}) - \hat{L}(\pmb{w}^*) +  \hat{L}(\pmb{w}^*) - L(\pmb{w}^*)
 \end{equation}
 By \eqref{eq:subset}, $\hat{L}(\pmb{\hat{w}}) - \hat{L}(\pmb{w}^*) \leq 0$ with probability $1-2\delta$. Thus, with probability at least $1-2\delta$, we have, 
 
\begin{equation}
    L(\pmb{\hat{w}}) -  L(\pmb{w}^*) \leq  L(\pmb{\hat{w}}) - \hat{L}(\pmb{\hat{w}})  +  \hat{L}(\pmb{w}^*) - L(\pmb{w}^*).
\end{equation}
Therefore, under assumption \ref{assump:learnable}, we can conclude with probability at least $1-6\delta$, $L(\pmb{\hat{w}}) -  L(\pmb{w}^*) \leq 2B(\delta,n,\mathcal{F})$. In addition, by \eqref{eq:ineq}, with probability at least $1-2\delta$, we have, 

\begin{eqnarray*}
 |L_0(\pmb{\hat{w}}) - L_1(\pmb{\hat{w}})| &\leq& B(\delta,n_0,\mathcal{F}) + B(\delta,n_1,\mathcal{F}) + |\hat{L}_0(\pmb{w}) - \hat{L}_1(\pmb{w})|  \nonumber \\
 &\leq& \hat{\gamma} + B(\delta,n_0,\mathcal{F}) + B(\delta,n_1,\mathcal{F})\\ &=& \gamma + 2B(\delta,n_0,\mathcal{F}) + 2B(\delta,n_1,\mathcal{F})
\end{eqnarray*}

\textbf{Proof [Theorem \ref{Theo:1}]}

We prove the theorem by contradiction. Assume $L_0(\pmb{w}^*) > \gamma$ and $L_1(\pmb{w}^*) > \gamma$ and $\pmb{\tilde{w}}$ is a feasible point of optimization \eqref{eq:BGLopt}.  Note that $\pmb{\tilde{w}}$ is a feasible point for optimization problem \eqref{eq:mainOP} as well. Since both $L_0(\pmb{w}^*)$ and $L_1(\pmb{w}^*)$ are larger than $\gamma$, we have,
\begin{eqnarray}
\E \{l(Y,f_{\pmb{w}^*})\} &=& \textstyle\sum_{a\in\{0,1\}} \Pr\{A=a\} L_a(\pmb{w}^*) > \gamma, \nonumber \\
\E \{l(Y,f_{\pmb{\tilde{w}}})\} &=& \textstyle\sum_{a\in\{0,1\}}\Pr\{A=a\} L_a(\pmb{\tilde{w}}) \leq \gamma.\nonumber 
\end{eqnarray}
It implies that $\pmb{w}^*$ cannot \ma{be} the solution to \eqref{eq:mainOP} because $\pmb{\tilde{w}}$ achieve smaller loss compared to $\pmb{w}^*$. \ma{This contradiction proves that the optimization problem \eqref{eq:BGLopt} cannot have a feasible point.}
%This is a contradiction, and optimization problem \eqref{eq:BGLopt} does not hav

\begin{proof}[Theorem \ref{Theo:2}]
Let $\pmb{\tilde{w}}$ be a feasible point of optimization problem \eqref{eq:BGLopt}, then  $\pmb{\tilde{w}}$ is also a feasible point to \eqref{eq:mainOP}. If $\min\{L_0(\pmb{w}^*),L_1(\pmb{w}^*)\} > \gamma$, then we must have: $$L(\pmb{w}^*) > \gamma \geq L(\pmb{\tilde{w}}). $$ This is a contradiction because it implies that $\pmb{w}^*$ is not an optimal solution to \eqref{eq:mainOP}. Therefore, $\min\{L_0(\pmb{w}^*),L_1(\pmb{w}^*)\}  \leq \gamma$. Similarly, we can prove $\max\{L_0(\pmb{w}^*),L_1(\pmb{w}^*)\}  \leq 2\gamma$ by contradiction. Specifically, if $\max\{L_0(\pmb{w}^*),L_1(\pmb{w}^*)\}  > 2\gamma$. Then, we have:  $$\max\{L_0(\pmb{w}^*),L_1(\pmb{w}^*)\} - \min\{L_0(\pmb{w}^*),L_1(\pmb{w}^*)\}  > \gamma,$$ which shows that $\pmb{w}^*$ is not a feasible point for \eqref{eq:mainOP}. This is a contradiction. Therefore,  $\max\{L_0(\pmb{w}^*),L_1(\pmb{w}^*)\} \leq 2\gamma$. 
\end{proof}
\subsection{Additional Experiments}

In this part, we compare performance of Algorithm 3 with Algorithm 2. As we know, Algorithm 3 finds a sub-optimal solution to \eqref{eq:mainOP}. 

\textbf{Adult Income Dataset:} We use the same dataset and the same parameter used in section 6.1. Note that

\begin{table}[h]
\centering
\resizebox{\linewidth}{!}{
\begin{tabular}{ccccccc} 
\toprule
& &$\gamma =0$ &  $\gamma = 0.1$ \\
\midrule
&training $L_0$ 	& 0.4516\pm 0.0004&   0.4045\pm 0.0005 \\
&training $L_1$ 	& 0.4577 \pm  0.0008&   0.4347\pm 0.0007  \\
&training $L$ 	&  0.4570\pm 0.0008 &  0.4315\pm 0.0003   \\
&test $L_0$ 	&0.4507\pm 0.0027  & 0.4130\pm 0.0044 \\
&test $L_1$ 	& 0.4562 \pm 0.0009 &  0.4288 \pm 0.0012 \\
\rot{\rlap{~Algorithm 2}}
&test $L$ 	& 0.4556\pm 0.0005 & 0.4270\pm 0.0006   \\
\midrule\\
&training $L_0$ 	& 0.4668\pm 0.0018 &   0.3650\pm 0.0019 \\
&training $L_1$ 	& 0.4657\pm 0.0020 & 0.4650\pm 0.0020  \\
&training $L$ 	& 0.4667\pm 0.0018  &  0.4541\pm 0.0020   \\
&test $L_0$ 	& 0.4598\pm 0.0062 & 0.3617\pm 0.0245 \\
&test $L_1$ 	& 0.4680\pm 0.0169 & 0.4665\pm 0.0142 \\ 
&test $L$ 	& 0.4671 \pm 0.0040 &  0.4550\pm 0.0041  \\\rot{\rlap{~Algorithm 3}} \\\bottomrule 
\end{tabular}}
	\caption{Logistic Regression model under \textsf{EL} fairness. }
\label{Table3}

\end{table}

As we can observe, Algorithm 3 finds a sub optimal solution under EL fairness. However, the performance under Algorithm 3 is similar the loss values under Algorithm 2.

 \textbf{Law School Admission Dataset:} In this part, we use the Law School Admission Dataset to compare Algorithm 2 with Algorithm 3 (Table \ref{Table4}). We use the same parameter as section 6.2. In particular, we set $R(\w) = 0.01 ||\w||^2$ and $\epsilon = 0.01$, and repeat the experiment for 5 times. We use the MSE loss as the loss function. As we can see in Table  \ref{Table4}, for the MSE loss, Algorithm 2 and Algorithm 3 have the similar performance. Even though Algorithm 3 finds a sub optimal solution, the training and test loss under Algorithm 3 is close to the training and test loss under algorithm 2. 
 
\begin{table}[h]
\centering
\resizebox{\linewidth}{!}{
\begin{tabular}{ccccccc} 
\toprule
& &$\gamma =0$ &$\gamma = 0.1$ \\
\midrule
&training $L_0$ 	& 0.7875\pm 0.0036 & 0.7859\pm 0.0018\\
&training $L_1$ 	& 0.7876\pm 0.0023 & 0.7778\pm 0.0024 \\
&training $L$ 	& 0.7876\pm 0.0024 &  0.7869\pm 0.0013 \\
&test $L_0$ 	& 0.7796\pm 0.0077 &  0.7778\pm 0.0071 \\
&test $L_1$ 	& 0.7863\pm 0.01013 & 0.7865\pm 0.0099 \\
\rot{\rlap{~Algorithm 2}}
&test $L$ 	& 0.7881\pm 0.0018 & 0.7826\pm 0.0053  \\
\midrule\\
&training $L_0$ 	&0.7878\pm 0.0021&  0.7886\pm 0.0024 \\
&training $L_1$ 	& 0.7888\pm 0.0024 &  0.7838\pm 0.0019 \\
&training $L$ 	& 0.7883\pm 0.0016 & 0.7865\pm 0.0013 \\
&test $L_0$ 	& 0.7798\pm 0.0082&   0.7759\pm 0.0072  \\
&test $L_1$ 	& 0.7866\pm 0.0103 &  0.7873\pm 0.0099 \\ 
&test $L$ 	&  0.7836\pm 0.0043 & 0.7822\pm 0.0053 \\\rot{\rlap{~Algorithm 3}} \\\bottomrule 
\end{tabular}}
	\caption{Linear Regression model under \textsf{EL} fairness. This table compares Algorithm 3 with Algorithm 2.  }
\label{Table4}
\end{table}
